# Supplementary material for: Efficient Waveform Capture without Absorption with Synthesis of Complex Frequencies
Source: arXiv:2512.17156 source file (2026-08-26)
Supplement: Supplementary file 1 [file SM.pdf]

Supplemental Material for

# Capturing Arbitrary Waveform without Absorption with Synthesis of Complex Frequencies

Zhaohua Tian,[1,2] Yu Tian,[1,3,*] Yadi Niu,[1] Qi Liu,[1,3] Zihan Mo,[1]
Haoyang Zhang,[1,6] Qihuang Gong,[1,3,4,5,6] and Ying Gu[1,3,4,5,6,†]

[1]*State Key Laboratory of Artificial Microstructure and Mesoscopic Physics & Department of Physics, Peking University, Beijing 100871, China*

[2]*Department of Physics, Zhejiang Sci-Tech University, Hangzhou 310018, China*

[3]*Frontiers Science Center for Nano-optoelectronics & Collaborative Innovation Center of Quantum Matter & Beijing Academy of Quantum Information Sciences, Peking University, Beijing 100871, China*

[4]*Collaborative Innovation Center of Extreme Optics, Shanxi University, Taiyuan, Shanxi 030006, China*

[5]*Peking University Yangtze Delta Institute of Optoelectronics, Nantong 226010, China*

[6]*Hefei National Laboratory, Hefei 230088, China*

(Dated: December 16, 2025)

**Contents**

1. Capture of superposition of two complex frequencies by a two-mode system 2

2. Integral representation of superpositions of complex frequencies 3

3. Proof of the equivalence between capture efficiency and synthesis fidelity 4
   3.1. Description of capture dynamics and efficiency 4
   3.2. Proof that only $f_{\mathrm{CF}}(\tau)$ can be captured 5
   3.3. Equivalence between capture efficiency and synthesis fidelity 7

4. Analytical scattering matrix zeros of a coupled-cavity chain system 8

5. Capture of five representative waveforms by a coupled-cavity chain system 9

6. Influence of the cavity parameter deviations on the capture efficiency 10

7. Influence of the cavity loss on the capture efficiency 11

References 12

* tian-yu@stu.pku.edu.cn
† ygu@pku.edu.cn

### 1. Capture of superposition of two complex frequencies by a two-mode system

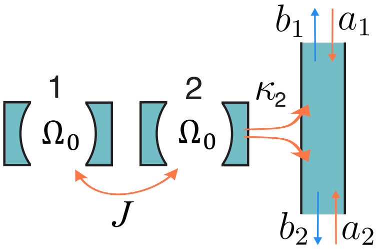


FIG. S1. Schematic of a scattering system consisting of two coupled cavities and a waveguide.

In the main text, Eq. (3) shows that for a system possessing multiple scattering-matrix zeros, arbitrary superpositions of these complex frequencies can be virtually perfectly absorbed. Here, we use a two-mode scattering system (Fig. S1) as a specific example to provide a more intuitive illustration. The two cavities share the same resonant frequency $\Omega_0$ and are coupled with strength $J$. Cavity 2 is side-coupled to a waveguide, interacting symmetrically with the two counter-propagating modes at a coupling rate of $\sqrt{\kappa_2/2}$. The Hamiltonian of the coupled-cavity system is

$$\mathbf{H} = \begin{pmatrix} \Omega_0 & J \\ J & \Omega_0 - i\kappa_2/2 \end{pmatrix}. \tag{1}$$

The scattering relation can be described by $|\boldsymbol{b}\rangle = \mathbf{S}(\tilde{\omega})|\boldsymbol{a}\rangle$, where $|\boldsymbol{a}\rangle = \begin{pmatrix} a_1 \\ a_2 \end{pmatrix}$, and $|\boldsymbol{b}\rangle = \begin{pmatrix} b_1 \\ b_2 \end{pmatrix}$ are the time-independent input and output amplitude vectors, respectively. The $2 \times 2$ scattering matrix takes the following form (detailed derivations can be found in Sec. 4 of this supplemental material)

$$\mathbf{S}(\tilde{\omega}) = \begin{pmatrix} 1 - \frac{i\kappa_2/2}{(\tilde{\omega}-\tilde{\omega}_1^*)(\tilde{\omega}-\tilde{\omega}_2^*)} & -\frac{i\kappa_2/2}{(\tilde{\omega}-\tilde{\omega}_1^*)(\tilde{\omega}-\tilde{\omega}_2^*)} \\ -\frac{i\kappa_2/2}{(\tilde{\omega}-\tilde{\omega}_1^*)(\tilde{\omega}-\tilde{\omega}_2^*)} & 1 - \frac{i\kappa_2/2}{(\tilde{\omega}-\tilde{\omega}_1^*)(\tilde{\omega}-\tilde{\omega}_2^*)} \end{pmatrix}, \tag{S1}$$

where

$$\begin{aligned} \tilde{\omega}_1 &= \Omega_0 + i\kappa_2/4 + \frac{\sqrt{16J^2 - \kappa_2^2}}{4}, \\ \tilde{\omega}_2 &= \Omega_0 + i\kappa_2/4 - \frac{\sqrt{16J^2 - \kappa_2^2}}{4}. \end{aligned} \tag{S2}$$

By solving the eigenvalue equation $\mathbf{S}(\tilde{\omega})|\boldsymbol{d}\rangle_m = \lambda_m|\boldsymbol{d}\rangle_m$, one can obtain the two eigenvalues $\lambda_1(\tilde{\omega}), \lambda_2(\tilde{\omega})$ and the corresponding eigenvectors $|\boldsymbol{d}\rangle_1, |\boldsymbol{d}\rangle_2$ as:

$$\begin{aligned} &\lambda_1(\tilde{\omega}) = 1, \quad |\boldsymbol{d}\rangle_1 = \frac{1}{\sqrt{2}}\begin{pmatrix} 1 \\ -1 \end{pmatrix}, \\ &\lambda_2(\tilde{\omega}) = \frac{(\tilde{\omega}-\tilde{\omega}_1)(\tilde{\omega}-\tilde{\omega}_2)}{(\tilde{\omega}-\tilde{\omega}_1^*)(\tilde{\omega}-\tilde{\omega}_2^*)}, \quad |\boldsymbol{d}\rangle_2 = \frac{1}{\sqrt{2}}\begin{pmatrix} 1 \\ 1 \end{pmatrix}. \end{aligned} \tag{S3}$$

The first eigenvalue $\lambda_1(\tilde{\omega}) = 1$ is frequency-independent and therefore cannot be used for light capture. Its eigenvector $|\boldsymbol{d}\rangle_1$ represents the antisymmetric input, where the two counter-propagating waves have equal amplitudes and a $\pi$ phase difference. This anti-symmetric excitation leads to destructive interference at the cavity–waveguide coupling interface, preventing the input from entering the coupled-cavity system. The second eigenvalue $\lambda_2(\tilde{\omega})$ possesses two distinct complex-frequency zeros:

$$\lambda_2(\tilde{\omega}_1) = 0, \qquad \lambda_2(\tilde{\omega}_2) = 0. \tag{S4}$$

Its eigenvector $|\boldsymbol{d}\rangle_2$ corresponds to the symmetric excitation, where waves from both sides have identical amplitudes and phases. For inputs prepared along the eigenvector $|\boldsymbol{d}\rangle_2$, each individual complex-frequency wave is perfectly and virtually absorbed:

$$\begin{aligned} \mathbf{S}(\tilde{\omega}_1)|\boldsymbol{d}\rangle_2 e^{-i\tilde{\omega}_1\tau} &= \lambda_2(\tilde{\omega}_1)|\boldsymbol{d}\rangle_2 e^{-i\tilde{\omega}_1\tau} = 0, \\ \mathbf{S}(\tilde{\omega}_2)|\boldsymbol{d}\rangle_2 e^{-i\tilde{\omega}_2\tau} &= \lambda_2(\tilde{\omega}_2)|\boldsymbol{d}\rangle_2 e^{-i\tilde{\omega}_2\tau} = 0. \end{aligned} \tag{S5}$$

Now consider an arbitrary superposition of the two complex frequencies,

$$f_{\mathrm{CF}}(\tau) = \alpha_1 e^{-i\tilde{\omega}_1\tau} + \alpha_2 e^{-i\tilde{\omega}_2\tau}, \tag{S6}$$

with superposition coefficients $\alpha_1$ and $\alpha_2$. When injected along $|\boldsymbol{d}\rangle_2$, the corresponding output is

$$\begin{aligned} \mathbf{S}(\tilde{\omega})\big(|\boldsymbol{d}\rangle_2 f_{\mathrm{CF}}(\tau)\big) &= \alpha_1\mathbf{S}(\tilde{\omega}_1)|\boldsymbol{d}\rangle_2 e^{-i\tilde{\omega}_1\tau} + \alpha_2\mathbf{S}(\tilde{\omega}_2)|\boldsymbol{d}\rangle_2 e^{-i\tilde{\omega}_2\tau} \\ &= \alpha_1\lambda_2(\tilde{\omega}_1)|\boldsymbol{d}\rangle_2 e^{-i\tilde{\omega}_1\tau} + \alpha_2\lambda_2(\tilde{\omega}_2)|\boldsymbol{d}\rangle_2 e^{-i\tilde{\omega}_2\tau} \\ &= 0. \end{aligned} \tag{S7}$$

Therefore, arbitrary superposition of the two complex-frequency waves is also virtually perfectly absorbed. As shown in Eq. (3) of the main text, the result obtained in this specific example can be generalized to a generic system supporting $N$ scattering-matrix zeros ($N > 2$), in which arbitrary superpositions of these complex frequencies can be perfectly captured.

## 2. Integral representation of superpositions of complex frequencies

We provide additional explanations of the integral representation for the superposition of complex frequencies. As illustrated in Fig. 2(b) of the main text, we consider an input waveform with a central frequency $\Omega_0$ and spectral width $\Gamma_0$. When the scattering-matrix zeros (i.e., the complex frequencies $\tilde{\omega}_n$) are densely distributed around the central frequency $\Omega_0$ and extend over a range much broader than the spectral width $\Gamma_0$, the discrete summation over complex frequencies converges to a contour integral. More explicitly, the distribution of complex frequencies should satisfy the following two conditions:

(C1) **Dense spacing:**

$$\frac{|\tilde{\omega}_n - \tilde{\omega}_{n-1}|}{\Gamma_0} \to 0.$$

This condition ensures that the spacing between adjacent complex frequencies is negligible compared to the spectral width of the input waveform, thereby suppressing the discretization error resulting from finite frequency sampling.

(C2) **Broad spectral extension:**

$$\frac{|\tilde{\omega}_N - \tilde{\omega}_1|}{\Gamma_0} \rightarrow \infty.$$

This condition requires the total spectral span of the complex-frequency distribution to be much wider than the waveform's spectral width, which minimizes truncation errors associated with a finite sampling range.

Under these two conditions (C1, C2), the discrete superposition $f_{\text{CF}}(\tau)$ converges to the contour integral

$$\begin{aligned} \lim_{\text{C1,C2}} f_{\text{CF}}(\tau) &= \lim_{\text{C1,C2}} e^{-i\Omega_0\tau} \sum_{n=1}^{N} \alpha(\tilde{\omega}_n) e^{-i(\tilde{\omega}_n - \Omega_0)\tau} \\ &= e^{-i\Omega_0\tau} \int_{C(s)} \tilde{\alpha}(s)\, e^{s\tau}\, ds, \end{aligned} \tag{S8}$$

which takes the form of an inverse Laplace transform [1]. Here, the integral variable $s = -i(\omega + i\gamma - \Omega_0)$ corresponds to the continuum limit of the densely distributed complex frequencies, shifted relative to $\Omega_0$. The contour $C(s)$ traced by these complex frequencies extends from $-\infty$ to $\infty$ along the $\omega$-axis. The coefficient $\tilde{\alpha}(s)$, representing the continuum limit of the discrete superposition coefficients, can be obtained directly from the Laplace transform of the target waveform: $\tilde{\alpha}(s) = \int_0^\infty f_{\text{Arb}}(\tau)\, e^{-s\tau}\, d\tau$. The representation in Eq. (S8) forms the mathematical foundation for synthesizing arbitrary waveforms using complex frequencies: since any arbitrary waveform $f_{\text{Arb}}(\tau)$ admits a Laplace transform $\tilde{\alpha}(s)$, it can always be synthesized through an appropriate distribution of complex frequencies specified by $\tilde{\alpha}(s)$.

## 3. Proof of the equivalence between capture efficiency and synthesis fidelity

In this section, we provide a proof of the equivalence between the capture efficiency ($\beta$) and the synthesis fidelity ($\mathcal{F}$). An energy-normalized waveform ($\int |f_{\text{Arb}}(\tau)|^2 \text{d}\tau = 1$) can be formally decomposed into two orthogonal components $f_{\text{Arb}}(\tau) = f_{\text{CF}}(\tau) + g(\tau)$, where $g(\tau)$ refers to the component that can't be superposed by finite number of complex frequencies. *The key to establishing this equivalence is to show that only the component $f_{CF}(\tau)$ can be captured.* In the following, we first introduce the temporal coupled-mode theory used to describe the capture dynamics and to compute $\beta$. Building on this, we then demonstrate that the captured energy is restricted to the component $f_{\text{CF}}(\tau)$. Finally, the equivalence between capture efficiency and synthesis fidelity is proved.

### 3.1. Description of capture dynamics and efficiency

In the main text, the scattering matrix approach is employed to illustrate the mechanism of capturing arbitrary waveforms (CAW). Here, we provide supplementary details using the temporal coupled-mode theory [2], which is required to obtain the exact capturing dynamics for arbitrary waveform inputs. The general coupled-mode equations can be written as :

$$i\partial_t|\psi(t)\rangle = \mathbf{H}|\psi(t)\rangle + \mathbf{D}^T|\mathcal{A}(t)\rangle, \tag{S9}$$

$$|\mathcal{B}(t)\rangle = |\mathcal{A}(t)\rangle - i\mathbf{D}|\psi(t)\rangle, \tag{S10}$$

where $|\mathcal{A}(t)\rangle = [\mathcal{A}_1(t), \mathcal{A}_2(t), ..., \mathcal{A}_N(t)]^T$, $|\mathcal{B}(t)\rangle = [\mathcal{B}_1(t), \mathcal{B}_2(t), ..., \mathcal{B}_N(t)]^T$ represent the time-dependent input and output amplitude vectors, respectively. $|\psi(t)\rangle = [c_1, c_2, ..., c_N(t)]^T$ is the system amplitude vector with $|c_n|^2$ represents the total energy of $n$-th cavity mode. The system coupling matrix $\mathbf{H} = \mathbf{\Omega} - i\mathbf{\Gamma}_\mathrm{C}/2 + \mathbf{J} - i\mathbf{K}/2$ includes the resonant frequencies $\mathbf{\Omega} = \mathrm{diag}(\Omega_1, \ldots, \Omega_N)$, the intrinsic loss $\mathbf{\Gamma}_\mathrm{C} = \mathrm{diag}(\Gamma_1, \ldots, \Gamma_N)$, the direct coherent coupling $\mathbf{J}$, and the indirect coupling $\mathbf{K}$ from $M$ open channels. Here $\mathbf{K}, \mathbf{\Omega}, \mathbf{\Gamma}_C$, and $\mathbf{J}$ are all real symmetric matrices. $\mathbf{D}$ is a real coupling matrix that connects the input/output channels with the system. For a lossless system, we have $\mathbf{\Gamma}_\mathrm{C} = 0$ and $\mathbf{D}^T\mathbf{D} = \mathbf{K}$ [3]. In general, the time dependence of the amplitude vectors $\mathcal{A}_n(t), \mathcal{B}_n(t)$ in different ports is different. In this research, we focus on the case where the input and output waveforms are identical across all ports. Consequently, the explicit time dependence of the input and output channels can be factored out:

$$|\mathcal{A}(t)\rangle = [\mathcal{A}_1(t), \mathcal{A}_2(t), ..., \mathcal{A}_N(t)]^T = |\boldsymbol{a}\rangle f_\mathrm{in}(t), \tag{S11}$$

$$|\mathcal{B}(t)\rangle = [\mathcal{B}_1(t), \mathcal{B}_2(t), ..., \mathcal{B}_N(t)]^T = |\boldsymbol{b}\rangle f_\mathrm{out}(t). \tag{S12}$$

where $f_\mathrm{in}(t)$ and $f_\mathrm{out}(t)$ represent the input and output waveforms. $|\boldsymbol{a}\rangle = [a_1, a_2, ..., a_N]^T$ and $|\boldsymbol{b}\rangle = [b_1, b_2, ..., b_N]^T$ denote the input and output time-independent amplitude vectors, respectively. The temporal coupled mode equations can be rewritten as follows

$$i\partial_t|\psi(t)\rangle = \mathbf{H}|\psi(t)\rangle + \mathbf{D}^T|\boldsymbol{a}\rangle f_\mathrm{in}(t), \tag{S13}$$

$$|\boldsymbol{b}\rangle f_\mathrm{out}(t) = |\boldsymbol{a}\rangle f_\mathrm{in}(t) - i\mathbf{D}|\psi(t)\rangle. \tag{S14}$$

For arbitrary waveform input $f_\mathrm{in}(t) = f_\mathrm{Arb}(t)$, the exact evolutions of $|\psi(t)\rangle$ as well as the captured energy $\langle\psi(t)|\psi(t)\rangle = \sum_{n=1}^{N} |c_n(t)|^2$ can both be obtained by numerically solving Eq. (S13). The capture efficiency is obtained by finding the maximum energy during the capture process $\beta = \mathrm{Max}_{t_0}\left[\langle\psi(t_0)|\psi(t_0)\rangle\right]$.

### 3.2. Proof that only $f_\mathbf{CF}(\tau)$ can be captured

With the temporal coupled-mode equations (S13) and (S14), we can show that only the components that are expandable in the complex-frequency basis can be captured, whereas the non-expandable residual component cannot. We begin by establishing the correspondence between the system eigenstates and the input complex frequencies. Consider the special case where the output vanishes, i.e., $|\boldsymbol{b}\rangle f_\mathrm{out}(t) = 0$. From the input–output relation in Eq. (S14), the input and cavity amplitudes are related by

$$|\boldsymbol{a}\rangle f_\mathrm{in}(t) = i\mathbf{D}|\psi(t)\rangle. \tag{S15}$$

Substituting Eq. (S15) into the coupled-mode equation Eq. (S13) yields

$$\begin{aligned} i\partial_t|\psi\rangle &= \mathbf{H}|\psi\rangle + \mathbf{D}^T|\boldsymbol{a}\rangle f_\mathrm{in}(t) \\ &= \mathbf{H}|\psi\rangle + \mathbf{D}^T i\mathbf{D}|\psi\rangle \\ &= (\mathbf{J} - i\mathbf{K}/2)|\psi\rangle + i\mathbf{K}|\psi\rangle \\ &= (\mathbf{J} + i\mathbf{K}/2)|\psi\rangle \\ &= \mathbf{H}^\dagger|\psi\rangle. \end{aligned} \tag{S16}$$

Thus, the capture dynamics without any scattering are governed by the non-Hermitian Hamiltonian $\mathbf{H}^\dagger$. Assuming that at time $t_0$ the system has completed capture without reflection, the evolution for $t \leq t_0$ is obtained via Eq. (S16) as

$$|\psi(t)\rangle = e^{-i\mathbf{H}^\dagger(t-t_0)}|\psi(t_0)\rangle\,\Theta(t_0 - t), \tag{S17}$$

where $\Theta$ denotes the Heaviside step function. Using Eq. (S15), the corresponding input waveform $f_{\text{in}}(\tau)$ can be obtained

$$|\boldsymbol{a}\rangle f_{\text{in}}(\tau) = i\mathbf{D}|\psi(\tau)\rangle = i\mathbf{D}\,e^{-i\mathbf{H}^\dagger(\tau-t_0)}|\psi(t_0)\rangle\,\Theta(t_0 - \tau). \tag{S18}$$

Consequently, for a complete capture there is a strict one-to-one correspondence between the incoming waveform $f_{\text{in}}(\tau)$ and the system state $|\psi(t_0)\rangle$ that stores the energy. By energy conservation, the total energy carried by the input equals the energy stored in the system after capturing:

$$\int_{-\infty}^{\infty} |f_{\text{in}}(\tau)|^2 \mathrm{d}\tau = \langle\psi(t_0)|\psi(t_0)\rangle \tag{S19}$$

Next, we show that this correspondence remains valid for complex frequencies and eigenstates. Let $\{|\psi_n\rangle\}$ and $\{\tilde{\omega}_n\}$ be the right eigenvectors and eigenvalues of $\mathbf{H}^\dagger$:

$$\mathbf{H}^\dagger|\psi_n\rangle = \tilde{\omega}_n|\psi_n\rangle. \tag{S20}$$

The non-Hermitian nature of $\mathbf{H}$ generally leads to nonorthogonal eigenvectors, i.e., $\langle\psi_m|\psi_n\rangle \neq \delta_{m,n}$ [4]. To expand an arbitrary system state in terms of these nonorthogonal eigenvectors, one can introduce a dual basis $|\phi_n\rangle$ defined as $|\phi_n\rangle = \sum_m (\mathbf{G}^{-1})_{n,m}|\psi_m\rangle$, where $\mathbf{G}_{m,n} = \langle\psi_m|\psi_n\rangle$ is the element of the Gram matrix [5]. In this way, the two sets of basis vectors satisfy the biorthogonality condition $\langle\phi_m|\psi_n\rangle = \delta_{m,n}$. The propagator admits the spectral expansion

$$e^{-i\mathbf{H}^\dagger(t_0-\tau)} = \sum_n |\psi_n\rangle\langle\phi_n|\,e^{-i\tilde{\omega}_n(t_0-\tau)}. \tag{S21}$$

According to Eq. (S18), if the system is prepared in eigenstate $|\psi_n\rangle$ at $t_0$, the input that excites this eigenstate is

$$\begin{aligned}
|\boldsymbol{a}\rangle f_{\text{in}}(\tau) &= i\mathbf{D}\,e^{-i\mathbf{H}^\dagger(\tau-t_0)}|\psi_n\rangle\,\Theta(t_0-\tau) \\
&= i\mathbf{D}\sum_{m=1}^{N}|\psi_m\rangle\langle\phi_m|\psi_n\rangle e^{-i\tilde{\omega}_m(t_0-\tau)}\Theta(t_0-\tau) \\
&= i\mathbf{D}\,|\psi_n\rangle\,e^{-i\tilde{\omega}_n(t_0-\tau)}\,\Theta(t_0-\tau) \\
&= |x\rangle\,\frac{1}{\sqrt{2\gamma_n}} f_n(\tau, t_0),
\end{aligned} \tag{S22}$$

where $|x\rangle \equiv i\mathbf{D}|\psi_n\rangle$ and

$$f_n(\tau, t_0) = \sqrt{2\gamma_n}\,e^{-i\tilde{\omega}_n(t_0-\tau)}\,\Theta(t_0-\tau), \tag{S23}$$

is the normalized complex-frequency basis function (with $\gamma_n$ chosen so that $\int |f_n(\tau, t_0)|^2 \mathrm{d}\tau = 1$). Thus a perfect excitation of eigenstate $|\psi_n\rangle$ corresponds precisely to an input waveform at the complex frequency $\tilde{\omega}_n$:

$$f_n(\tau, t_0) \longleftrightarrow |\psi_n\rangle. \tag{S24}$$

Linearity implies that arbitrary superposition of the complex frequencies $f_{\rm CF}(\tau)$ excites the corresponding superposition of eigenstates $|\psi_{\rm CF}\rangle$:

$$f_{\rm CF}(\tau)=\sum_n \alpha_n f_n(\tau,t_0)\longleftrightarrow|\psi_{\rm CF}\rangle=\sum_n\alpha_n|\psi_n\rangle. \tag{S25}$$

By energy conservation, the total energy carried by the input $f_{\rm CF}(\tau)$ equals the energy stored in the system after capturing:

$$\int_{-\infty}^{\infty}|f_{\rm CF}(\tau)|^2{\rm d}\tau=\langle\psi_{\rm CF}|\psi_{\rm CF}\rangle \tag{S26}$$

Having established the correspondence between superpositions of complex frequencies and the system eigenstates that store them, we now prove by contradiction that the remaining component $g(\tau)$ of the input waveform cannot be captured. Assume that the unexpandable residual $g(\tau)$ could also be captured. The corresponding captured state $|\psi_g\rangle$ is obtained by solving Eq. (S13) as

$$|\psi_g\rangle=\int_{-\infty}^{t_0}e^{-i\mathbf{H}(t_0-\tau)}(-i\mathbf{D}^T)|\mathbf{a}\rangle g(\tau)\,{\rm d}\tau=\int_{-\infty}^{\infty}e^{-i\mathbf{H}(t_0-\tau)}(-i\mathbf{D}^T)|\mathbf{a}\rangle g(\tau)\Theta(t_0-\tau)\,{\rm d}\tau. \tag{S27}$$

It can be readily shown that the resulting state $|\psi_g\rangle$ is orthogonal to each eigenstate $|\psi_n\rangle$:

$$\begin{aligned}\langle\psi_n|\psi_g\rangle&=\langle\psi_n|\int_{-\infty}^{\infty}e^{-i\mathbf{H}(t_0-\tau)}(-i\mathbf{D}^T)|\mathbf{a}\rangle g(\tau)\Theta(t_0-\tau)\,{\rm d}\tau\\&=\int_{-\infty}^{\infty}[\,i\mathbf{D}e^{-i\mathbf{H}^\dagger(\tau-t_0)}|\psi_n\rangle\Theta(t_0-\tau)\,]^\dagger|\mathbf{a}\rangle g(\tau)\,{\rm d}\tau\\&=\int[\,|x\rangle f_n(\tau-t_0)\,]^\dagger g(\tau)|a\rangle\,{\rm d}\tau\\&=\langle x|a\rangle\int_{-\infty}^{\infty}f_n^*(\tau,t_0)\,g(\tau)\,{\rm d}\tau=0,\end{aligned} \tag{S28}$$

where in the third line of Eq. (S28), we have used the one-to-one correspondence between the complex frequencies and the system eigenstates, as established in Eq. (S22). In the last line, we have employed the fact that the complex-frequency non-expandable part $g(\tau)$ is orthogonal to every complex-frequency basis $f_n$:

$$\int f_n(\tau,t_0)\,g^*(\tau)\,{\rm d}\tau=0\quad\text{for all }n. \tag{S29}$$

Owing to the completeness of the system eigenstates, no state within the constructed system can be orthogonal to all eigenstates simultaneously. Hence, $|\psi_g\rangle=0$. Therefore, only the complex-frequency–expandable component $f_{\rm CF}(\tau)$ of an input waveform can be captured, while the non-expandable part $g(\tau)$ cannot.

### 3.3. Equivalence between capture efficiency and synthesis fidelity

We define the synthesis fidelity as the proportion of the waveform that is expandable in complex frequencies:

$$\mathcal{F}=\int|f_{\rm CF}(\tau)|^2\,d\tau. \tag{S30}$$

In addition, the capture efficiency ($\beta$) is characterized by the maximum energy stored in the system during the capture process. For arbitrary waveform input, it has been proved that only the component $f_{\mathrm{CF}}(\tau)$ can be captured, and the remaining part $g(\tau)$ cannot. According to Eq. (S25) and (S26), after capture, the energy carried by the capturable component $f_{\mathrm{CF}}(\tau)$ is completely stored in the system as the state $|\psi_{\mathrm{CF}}\rangle$. Therefore, the capture efficiency is given by

$$\beta = \langle\psi_{\mathrm{CF}}|\psi_{\mathrm{CF}}\rangle = \int |f_{\mathrm{CF}}(\tau)|^2 \, d\tau. \tag{S31}$$

Hence,

$$\mathcal{F} = \beta. \tag{S32}$$

Consequently, the capture efficiency of an arbitrary waveform is equal to its synthesis fidelity by complex frequencies.

### 4. Analytical scattering matrix zeros of a coupled-cavity chain system

For the uniform coupled-cavity chain structure presented in Fig. 3(a) of the main text, an analytical expression for the scattering matrix zeros can be obtained. The scattering dynamics are described by the temporal-coupled-mode equation (S13), with the Hamiltonian taking the following tridiagonal form:

$$\mathbf{H} = \begin{pmatrix} \Omega_0 & J & & \\ J & \Omega_0 & \ddots & \\ & \ddots & \ddots & J \\ & & J & \Omega_0 - i\kappa_N/2 \end{pmatrix}. \tag{S33}$$

Only the $N$-th cavity interacts symmetrically with the waveguide, therefore, the corresponding coupling matrix $\mathbf{D}$ connecting the input/output channels to the system is

$$\mathbf{D} = \begin{pmatrix} 0 & 0 & \cdots & \sqrt{\kappa_N/2} \\ 0 & 0 & \cdots & \sqrt{\kappa_N/2} \end{pmatrix}. \tag{S34}$$

Considering a monochromatic input waveform $f_{\mathrm{in}}(\tau) = e^{-i\tilde{\omega}\tau}$, the scattering matrix can be obtained from the coupled-mode equations (S13) and (S14) as [2]

$$\mathbf{S}(\tilde{\omega}) = \mathbf{I}_M - i\mathbf{D}(\tilde{\omega}\mathbf{I}_N - \mathbf{H})^{-1}\mathbf{D}^T = \mathbf{I}_M - i\mathbf{D}\mathbf{T}^{-1}\mathbf{D}^T. \tag{S35}$$

Here, $\mathbf{T} = \tilde{\omega}\mathbf{I}_N - \mathbf{H}$ is also a tridiagonal matrix, and $\mathbf{I}_M$ and $\mathbf{I}_N$ denote the $M$- and $N$-dimensional identity matrices, respectively. According to the specific structure of $\mathbf{D}$, it is unnecessary to compute every element of the inverse matrix $\mathbf{T}^{-1}$. Only the $(N, N)$-th element is relevant, and it can be expressed analytically as [6]

$$(\mathbf{T}^{-1})_{N,N} = \frac{1}{\det(\mathbf{T})} = \frac{1}{\prod_{n=1}^{N}(\tilde{\omega} - \tilde{\omega}_n^*)}. \tag{S36}$$

Here, $\tilde{\omega}_n^*$ denotes the eigenvalue of $\mathbf{H}$. Substituting this result into Eq. (S35), the scattering matrix can be written in the analytical form,

$$\mathbf{S}(\tilde{\omega}) = \mathbf{I}_M - i\mathbf{D}\mathbf{T}^{-1}\mathbf{D}^T$$

$$
\begin{aligned}
&= \mathbf{I}_M - \frac{i\kappa_N/2}{\prod_{n=1}^{N}(\tilde{\omega}-\tilde{\omega}_n^*)}\begin{pmatrix}1 & 1\\ 1 & 1\end{pmatrix} \\
&= \begin{pmatrix} 1-\dfrac{i\kappa_N/2}{\prod_{n=1}^{N}(\tilde{\omega}-\tilde{\omega}_n^*)} & -\dfrac{i\kappa_N/2}{\prod_{n=1}^{N}(\tilde{\omega}-\tilde{\omega}_n^*)} \\ -\dfrac{i\kappa_N/2}{\prod_{n=1}^{N}(\tilde{\omega}-\tilde{\omega}_n^*)} & 1-\dfrac{i\kappa_N/2}{\prod_{n=1}^{N}(\tilde{\omega}-\tilde{\omega}_n^*)} \end{pmatrix}.
\end{aligned} \tag{S37}
$$

The two eigenvalues of the scattering matrix $\mathbf{S}(\tilde{\omega})$ and their eigenvectors are:

$$
\lambda_1(\tilde{\omega}) = 1, \quad |\boldsymbol{d}\rangle_1 = \frac{1}{\sqrt{2}}\begin{pmatrix}1\\ -1\end{pmatrix}, \tag{S38}
$$

$$
\begin{aligned}
\lambda_2(\tilde{\omega}) &= 1 - \frac{i\kappa_N}{\prod_{n=1}^{N}(\tilde{\omega}-\tilde{\omega}_n^*)} = \frac{\prod_{n=1}^{N}(\tilde{\omega}-\tilde{\omega}_n)}{\prod_{n=1}^{N}(\tilde{\omega}-\tilde{\omega}_n^*)}, \\
|\boldsymbol{d}\rangle_2 &= \frac{1}{\sqrt{2}}\begin{pmatrix}1\\ 1\end{pmatrix}.
\end{aligned} \tag{S39}
$$

Here, $\lambda_1 = 1$ is independent of the input frequency and cannot be used for light capture. In contrast, $\lambda_2(\tilde{\omega})$ possesses $N$ complex-frequency zeros $\{\tilde{\omega}_n\}$ and can therefore be used for CAW. Its corresponding eigenvector $|\boldsymbol{d}\rangle_2$ indicates that the waveform should be injected from both sides of the waveguide with equal amplitudes and phases.

Meanwhile, the zeros of $\lambda_2(\tilde{\omega})$ coincide with the eigenvalues of the non-Hermitian Hamiltonian $\mathbf{H}^\dagger$. Therefore, by engineering $\mathbf{H}$, one can precisely control the distribution of these complex-frequency zeros. For the uniform coupled-cavity system shown in Fig. 3(a) of the main text, in the absence of waveguide coupling ($\kappa_N = 0$), the eigenvalues of $\mathbf{H}^\dagger$ are $\tilde{\omega}_n = \Omega_0 + 2J\cos\left(\frac{n\pi}{N+1}\right)$, which are non-uniformly distributed within $(\Omega_0 - 2J, \Omega_0 + 2J)$. When waveguide coupling $\kappa_N$ is introduced, these eigenvalues acquire imaginary parts, while their real parts shift only slightly, remaining largely confined within the interval $(\Omega_0 - 2J,\ \Omega_0 + 2J)$. Thus, by properly engineering $J$ and $\kappa_N$, one can effectively control the distribution of the complex frequencies. As shown in Fig. 3(b) of the main text, we set $\kappa_N = 2J$ and $J = 0.2\,\Gamma_0 N$, such that the complex frequencies gradually extend and spread around $\Omega_0$ as the number of cavities $N$ increases.

### 5. Capture of five representative waveforms by a coupled-cavity chain system

We provide additional details on the calculations of capture efficiency for five representative input waveforms: exponentially decaying ($f_{\mathrm{ED}}(\tau)$), rectangular ($f_{\mathrm{Rect}}(\tau)$), triangular ($f_{\mathrm{Tri}}(\tau)$), Gaussian ($f_{\mathrm{Gau}}(\tau)$), and a randomly shaped waveform $f_{\mathrm{Rdm}}(\tau)$. All waveforms are

energy-normalized and take the following analytical forms:

$$\begin{aligned}
f_{\mathrm{ED}}(\tau) &= \sqrt{\Gamma_0} e^{-\Gamma_0 \tau/2 - i\Omega_0 \tau}\Theta(\tau), \\
f_{\mathrm{Gau}}(\tau) &= \sqrt{\frac{\Gamma_0}{\pi}} e^{-\Gamma_0^2 \tau^2/2 - i\Omega_0 \tau}, \\
f_{\mathrm{Rect}}(\tau) &= \sqrt{3\Gamma_0} e^{-i\Omega_0 \tau}\Theta\left(\frac{1}{3\Gamma_0} - \tau\right)\Theta(\tau), \\
f_{\mathrm{Tri}}(\tau) &= \sqrt{3 \times (3\Gamma_0)^3} \tau e^{-i\Omega_0 \tau}\Theta\left(\frac{1}{3\Gamma_0} - \tau\right)\Theta(\tau), \\
f_{\mathrm{Rdm}}(\tau) &= \frac{1}{\sqrt{N_{\mathrm{nor}}}}\left[f_{\mathrm{ED}}(\tau) + f_{\mathrm{Gau}}(\tau) + f_{\mathrm{Rect}}((\tau) + f_{\mathrm{Tri}}(\tau)\right],
\end{aligned} \tag{S40}$$

where $\Gamma_0$ and $\Omega_0$ denote the spectral width and central frequency of input waveforms. The random-shaped waveform $f_{\mathrm{Rdm}}(\tau)$ is a superposition of the other four waveforms, with $N_{\mathrm{nor}}$ being the normalization coefficients. For each waveform, we numerically solve Eq. (S13) to obtain the exact evolutions of the captured energy $\langle\psi(t)|\psi(t)\rangle$. The capture efficiency is obtained by finding the maximum energy during the capture process $\beta = \mathrm{Max}_{t_0}\left[\langle\psi(t_0)|\psi(t_0)\rangle\right]$. The capture efficiencies for five input waveforms as a function of the cavity numbers are presented in Fig. 3(c) of the main text.

### 6. Influence of the cavity parameter deviations on the capture efficiency

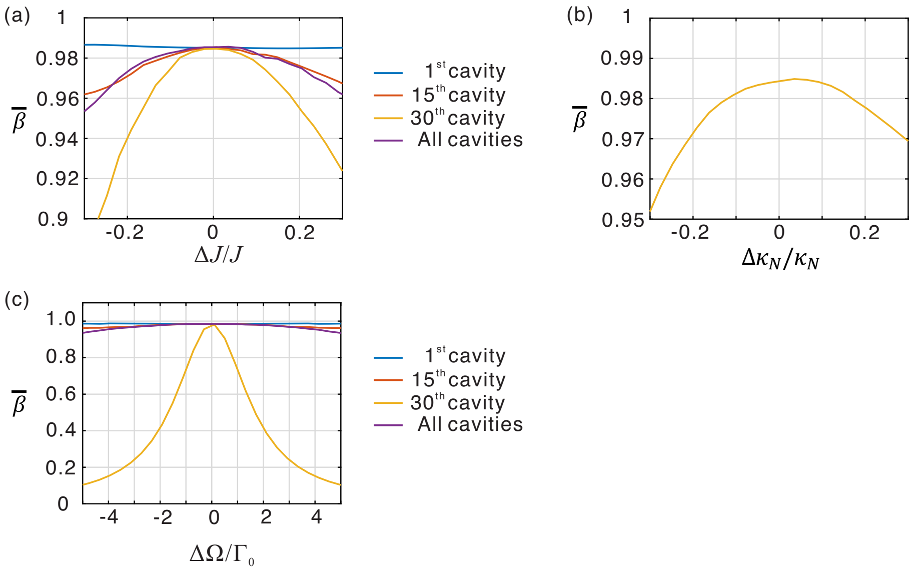


FIG. S2. Influence of cavity parameter deviations on average capture efficiency. The average capture efficiency $\bar{\beta}$ for five representative input waveforms is evaluated as a function of deviations in (a) the inter-cavity coupling $\Delta J/J$, (b) the coupling between the terminal cavity and the waveguide $\Delta\kappa_N/\kappa_N$, and (c) the cavity resonance frequency $\Delta\Omega/\Gamma_0$. Deviations are introduced individually in the first cavity (blue solid line), the 15-th cavity (orange), and the terminal cavity connected to the waveguide (yellow), as well as a uniform deviation applied to all cavities in the chain (purple).

When the coupling strengths deviate from the designed value, there will be a corresponding shift in the distribution of scattering matrix zeros. This will influence the performance of waveform synthesis by complex frequencies, leading to the decrease in capture efficiency. To quantify this effect, we take the uniform cavity chain in Fig. 3 of main text with $N = 30$ as an example. The average efficiencies $\bar{\beta}$ as a function of cavity parameter deviations, including the inter-cavity coupling strength $J$ , cavity resonance frequency $\Omega$, and the coupling between the terminal cavity and the waveguide $\kappa_N$ are shown in Fig. S2 (a)-(c).

**Influence of deviations in $J$.** The inter-cavity coupling $J$ is essential for establishing the desired distribution of complex frequencies. As shown in Fig. S2(a), we first examine the effect of deviations in the coupling strength $J_{m,m+1}$ at specific positions along the uniform chain: the first cavity ($J_{1,2}$, blue), the middle cavity ($J_{15,16}$, orange), and the terminal cavity near the waveguide ($J_{28,29}$, yellow). One sees that in all cases, deviations exhibit only minor reductions in $\bar{\beta}$. Additionally, coupling strength deviations near the waveguide produce a slightly larger decrease in capture efficiency. This is because deviations in the coupling strength $J$ at the terminal cavity hinder the efficient excitation of the subsequent cavities and the entire chain, leading to a more pronounced reduction in the overall waveform-capture efficiency. We also examine the case where the coupling strength of all cavities deviates from the designed value. As indicated by the purple solid line in Fig. S2(a), even when $J$ deviates by as much as 30% from its optimal value, the average capture efficiency drops by less than 3%, demonstrating the excellent robustness of the proposed scheme against coupling strength deviations.

**Influence of deviations in $\kappa_N$.** A proper value of $\kappa_N$ is also important for achieving the desired distribution of scattering matrix zeros. In the main text, we set $\kappa_N = 2J$. As shown in Fig. S2(b), a deviation of $\kappa_N$ from its designed value leads to a small reduction in the capture efficiency. Specifically, for a 30% relative deviation of coupling strength $\kappa_N$, the efficiency reduction remains below 3%, confirming the robustness of the scheme to moderate variations in $\kappa_N$.

**Influence of cavity detuning $\Delta\Omega_C = \Omega - \Omega_0$.** Finally, we investigate the influence of cavity detuning on the capture efficiency. As shown in Fig. S2(c), we consider both the detuning of individual cavities at specific positions and uniform detuning across the entire chain. The detuning of the cavity closest to the waveguide exhibits the strongest impact, since detuning at this site prevents the waveform from efficiently entering the system. In contrast, detuning of intermediate cavities or detuning across all cavities leads to only minor degradation. Overall, the influence of cavity detuning on the capture efficiency is mild. A uniform detuning of $2\Gamma_0$ causes a drop of the efficiency of less than 1%. In practical implementations, such detuning can be readily compensated through photoinduced resonance tuning, electro-optic tuning, post-fabrication trimming, or MEMS actuation [7–10].

## 7. Influence of the cavity loss on the capture efficiency

The proposed mechanism of CAW relies on the construction of a series of complex-frequency zeros in a lossless structure. The presence of loss leads to the dissipation of the captured wave, thereby reducing the capture efficiency. To quantify this, we calculate the influence of cavity loss on the average capture efficiency $\bar{\beta}$ for five representative waveforms. We take the uniform coupled-cavity structure shown in Fig. 3(a) of the main text with $N = 30$ as an example. We first examine the cases where only one cavity, located at the beginning (blue solid line), the middle (orange), or the end of the chain (yellow), has a loss

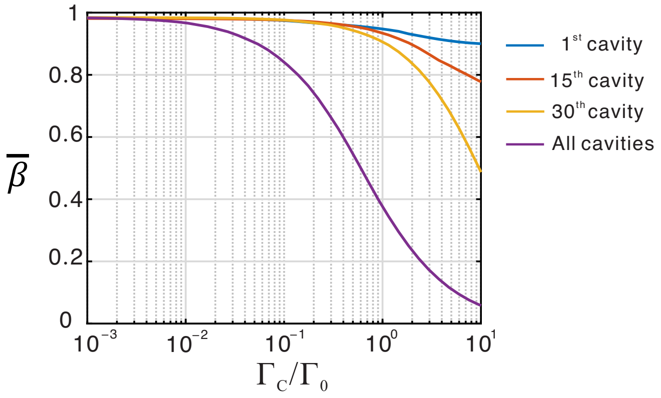


FIG. S3. Influence of cavity loss $\Gamma_C/\Gamma_0$ on the average capture efficiency. Loss is introduced individually in the first cavity (blue solid line), the 15-th cavity (orange), and the terminal cavity coupled to the waveguide (yellow), as well as uniformly across all cavities in the chain (purple).

of $\Gamma_C$ [Fig. S3]. When $\Gamma_C/\Gamma_0 < 0.1$, the reduction in capture efficiency remains below 1%. Thus, the loss of a single cavity has a negligible impact on the overall efficiency. Meanwhile, the cavity loss at the beginning of the chain causes a smaller drop than that at the terminal cavity near to the waveguide.

We further examine the scenario in which all cavities exhibit identical losses (purple solid line in Fig. S3). The results indicate that as long as $\Gamma_C/\Gamma_0 < 0.01$, the average capture efficiency remains nearly unaffected. While for $\Gamma_C/\Gamma_0 < 0.1$, the average efficiency stays around 85%. Therefore, cavity loss is a critical factor influencing waveform capture and should be minimized as much as possible. As an example, consider the capture of nanosecond pulse with a wavelength of 800 nm and a lifetime of 10 ns, corresponding to a linewidth of about $\Gamma_0/(2\pi)$ =3 GHz. Keeping the cavity loss $\Gamma_C/(2\pi)$ below 30 MHz ensures $\Gamma_C/\Gamma_0 < 0.01$, which corresponds to a quality factor of $\sim 10^7$. Such a $Q$ factor is readily attainable in state-of-the-art integrated photonic systems [11, 12].

---


[1] G. Arfken, H. Weber , and F. Harris. Mathematical methods for physicists: a comprehensive guide. (Academic Press, 2011)

[2] S. Fan, W. Suh , and J. Joannopoulos. Temporal coupled-mode theory for the Fano resonance in optical resonators. J. Opt. Soc. Am. A **20**, 569–572 (2003)

[3] A. Krasnok, D. Baranov, H. Li, M.-A. Miri, F. Monticone , and A. Alú. Anomalies in light scattering. Adv. Opt. Photon. **11**, 892–951 (2019)

[4] Y. Ashida, Z. Gong , and M. Ueda. Non-Hermitian physics. Adv. Phys. **69**, 249–435 (2020)

[5] K. Hoffman and R. Kunze. Linear Algebra. (Pearson India Education Services, 2015)

[6] C. Fonseca and J. Petronilho. Explicit inverses of some tridiagonal matrices. Linear Algebra Appl. **325**, 7–21 (2001)

[7] J. Wang, F. Bo, S. Wan, W. Li, F. Gao, J. Li, G. Zhang, and J. Xu. High-Q lithium niobate microdisk resonators on a chip for efficient electro-optic modulation. Opt. Express **23**, 23072–23078 (2015)

[8] A. Faraon, D. Englund, D. Bulla, B. Luther-Davies, B. Eggleton, N. Stoltz, P. Petroff , and J. Vučković. Local tuning of photonic crystal cavities using chalcogenide glasses. Appl. Phys.

Lett. **92**, 043123 (2008)

[9] M. Lee and M. Wu. Tunable coupling regimes of silicon microdisk resonators using MEMS actuators. Opt. Express **14**, 4703–4712 (2006)

[10] D. Sparacin, C.-H. Kimerling, L. Michel, J. Lock, and K. Gleason. Trimming of microring resonators by photo-oxidation of a plasma-polymerized organosilane cladding material. Opt. Lett. **30**, 2251–2253 (2005)

[11] X. Ji, F. Barbosa, S. Roberts, A. Dutt, J. Cardenas, Y. Okawachi, A. Bryant, A. Gaeta, and M. Lipson. Ultra-low-loss on-chip resonators with sub-milliwatt parametric oscillation threshold. Optica **4**, 619–624 (2017)

[12] W. Jin, Q. Yang, L. Chang, B. Shen, H. Wang, M. Leal, L. Wu, M. Gao, A. Feshali, M. Paniccia, K. Vahala, and J. Bowers. Hertz-linewidth semiconductor lasers using CMOS-ready ultra-high-Q microresonators. Nat. Photonics **15**, 346–353 (2021)
